# Supplementary material for: Continuous Geometry-Aware Graph Diffusion via Hyperbolic Neural PDE
Source: arXiv:2406.01282 source file (2024-06-07)
Supplement: Supplementary file 1 [file AppE.tex]

\section*{Appendix E: Additional Declaration for Experiments}
\subsection*{Low Label Rates Image-Text Classification}
% We additionally conducted experiments on the \textsc{CIFAR-10}, \textsc{STL-10}, and \textsc{20News-Group} datasets to test HGDE for standard classification tasks with limited label rates. In Appendix~E, Tab.~\ref{tb:image-text-cls} shows the testing accuracy of HGDE and its competitors, including MLP, ManiReg, GCN-kNN, GAT-kNN, DenseGAT, and GLCN. The two HGDE models outperform MLP in almost all cases, indicating the effectiveness of learning the interdependence between instances. Additionally, HGDE shows significant improvements over GCN and GAT, which are limited by the handcrafted graph and result in suboptimal propagation. Furthermore, HGDE performs significantly better than GLCN, a strong baseline that learns new (static) graph structures, demonstrating the superiority of our evolving diffusivity that can adapt to different layers.

We conducted additional experiments on the \textsc{CIFAR}, \textsc{STL}, and \textsc{20News} datasets to evaluate HGDE in multiple classification scenarios with limited label rates. We employ the SimCLR \cite{chen2020simclr} extracted embedding as provided in \cite{wu2023difformer} for image classification. For the pre-processed \textsc{20News} \cite{pedregosa2011scikit} for text classification, we take $10$ topics and regard words with $\text{TF-IDF} > 5$ as features. For graph-based models, we use \textit{k}NN to construct a graph over input features. For HGDE (hyperbolic), we map the initial feature to $\mathbb{D}_\kappa$ via $\exp_\mathbf{o}^\kappa(\cdot)$ before the embedding process. As depicted in Tab.~\ref{tb:image-text-cls}(Left), HGDE consistently surpasses its opponents, including MLP, LabelProp \cite{zhu2003semi}, ManiReg \cite{belkin2006manifold}, GCN-\textit{k}NN, GAT-\textit{k}NN, DenseGAT, and GLCN \cite{jiang2019semi}. Across all datasets, HGDE outperforms the Euclidean models, underscoring its proficiency in understanding the potential hierarchical structure of image embeddings \cite{khrulkov2020hyperbolic} and text embeddings. Furthermore, HGDE exhibits superior performance compared to static graph-based baselines \textit{e.g.,} GAT-\textit{k}NN and GLCN, which underlines the distinct advantage of the evolving diffusivity mechanism of HGDE, which dynamically adapts across different layers. 

% \subsection*{Memory and Runtime Comparison}
